# Supplementary material for: StepFun-Formalizer: Unlocking the Autoformalization Potential of LLMs through Knowledge-Reasoning Fusion
Source: arXiv:2508.04440 source file (2025-12-26)
Supplement: Supplementary file 1 [file RL_parameters.tex]

\begin{table*}[h]
\label{tab:rl_param}
\centering
\footnotesize
\begin{tabular}{lllll}
\hline
\textbf{Parameter Category} & \textbf{Parameter Name} & \textbf{Value} & \textbf{Parameter Name} & \textbf{Value} \\
\hline
\multirow{2}{*}{Batch Size Related} & Global Batch Size & 128 & Training Batch Size & 64 \\
& Dynamic Batch Size & True & & \\
\hline
\multirow{2}{*}{Rollout Configuration} & Rollout Number & 16 & Rollout Temperature & 1.0 \\
& Rollout Engine & VLLM & Rollout GPU Memory Utilization & 0.8 \\
\hline
\multirow{2}{*}{Optimization \& Regularization} & Learning Rate & $1 \times 10^{-6}$ & Weight Decay & 0.0 \\
& KL Coefficient & 0.0 & KL Loss Coefficient & 0.0 \\
\hline
\multirow{2}{*}{Clipping \& Penalty} & Clip Ratio (High) & 0.28 & Clip Ratio (Low) & 0.2 \\
& Overlong Penalty Factor & 1.0 & & \\
\hline
\multirow{2}{*}{Length Control} & Max Train Response Length (Full) & 16384 & Overlong Response Length & 1024 \\
& Max Generate Response Length & 32768 & & \\
\hline
\multirow{3}{*}{\parbox{3.5cm}{Computation \& \\ Memory Optimization}} & Gradient Clip & 0.5 & Gradient Checkpointing & True \\
& Use Liger Kernel & True & VLLM Enforce Eager & False \\
& Tensor Parallel Size & 4 & & \\
\hline
\multirow{1}{*}{Distributed Training Configuration} & Number of Nodes & 2 & GPUs per Node & 8 \\
\hline
\multirow{1}{*}{Data Processing} & Remove Padding & True & Token Level Loss & True \\
\hline
\multirow{1}{*}{FSDP Related} & FSDP Optimizer Offload & False & FSDP Parameter Offload & False \\
\hline
\end{tabular}
\caption{RL Parameter Setting.}
\end{table*}
