# Supplementary material for: StepFun-Formalizer: Unlocking the Autoformalization Potential of LLMs through Knowledge-Reasoning Fusion
Source: arXiv:2508.04440 source file (2025-12-26)
Supplement: Supplementary file 3 [file ablation_data_selection_effi.tex]

\begin{table}[h]
\fontsize{8}{11}\selectfont
\centering

\begin{tabular}{lcc}
\toprule
Method & Data Amount & Training Time (h) \\
\midrule
\rowcolor[rgb]{0.925,0.925,0.925} \xname (Ours)   & \textbf{182548}       & \textbf{17.5}   \\
w/o LLM selection   & 253913    &  21.8   \\
\bottomrule
\end{tabular}%
\caption{Efficiency comparison of with and without LLM selection in knowledge data distillation.}
\label{tab:ablation_data_selection_effi}
\end{table}
