# Supplementary material for: StepFun-Formalizer: Unlocking the Autoformalization Potential of LLMs through Knowledge-Reasoning Fusion
Source: arXiv:2508.04440 source file (2025-12-26)
Supplement: Supplementary file 4 [file sft_parameters.tex]

\begin{table*}[h]

\centering
\footnotesize
\begin{tabular}{lllll}
\hline
\textbf{Parameter Category} & \textbf{Parameter Name} & \textbf{Value} & \textbf{Parameter Name} & \textbf{Value} \\
\hline
\multirow{1}{*}{Training Mode} & Finetuning Type & Full Parameter & Deepspeed & Zero3 \\
\hline
\multirow{3}{*}{Optimization \& Scheduling} & Epochs & 2 & Learning Rate (LR) & $2 \times 10^{-5}$ \\
& Batch Size & 128 (Stage 1) / 8 (Stage 2) & Optimizer & AdamW \\
& LR Scheduler & Cosine Decay & LR Warmup Steps & 0 \\
& Numerical Precision & BF16 & & \\
\hline
\multirow{1}{*}{Context \& Data Handling} & Max Context Length & 16384 & Packing & False \\
\hline
\end{tabular}

\caption{SFT parameter setting.}
\label{tab:sft_param_1}

\end{table*}
